# Supplementary material for: MatCLIP: Light- and Shape-Insensitive Assignment of PBR Material Models
Source: arXiv:2501.15981 source file (2025-08-09)
Supplement: Supplementary file 1 [file appendix.tex]

\onecolumn
\section{Improvements}

\begin{verbatim}

Step 1:  Make a descriptor that works for retreival

We need a dataset of rendered objects with PBRs from MatSynth. 
- The datset should have masked regions and the MatSynth PBR used for each masked region. 
- For each masked-region we compute ImagGPY 1K histogram
- For each PBR we do same for diffuse map
- Can check retreival metrics. 
-   Try this on an RGB texture library [find one?]
- "...." comput patch-CLIP vector and overall image CLIP and save  for patch AND pbr textures
   - Consider AlphaCLIP
- Check retrival metrics
    - for ONLy CLIP and for concatenated CLIP+hist
- Cluster early conv layers of eg. vgg1
- Compute histgrams as above for renders and for diffuse PBR
- Chek retrival metrics
    - for CONLY conv and COncatenated

{Next Step will be training with contrastive loss on these to improve retreival metrics}

IMAgeGPT - Quantizes colors 1o 1K and makes histogram. 
JCF:  Cluster activations from early layers of a Convnet (e.g. VGG)  pretrained.  Make histogram. 
Concatenate:  SD Images CLIP, patch CLIP

IDEA: For a vector that captures useful texture info. 
- Train contrastive somehow to learn (smaller/better/more invariant) vector

Validate using retreival on MatSynth. 
  - Render with various lighting
  - Compare correct vs incorrect matsynth assignments
  - Input is from masked portion of rednered object. 

Get best results possible on fixed library. 


Idea I want to dismiss because I think it is hard
- take the rendered patch of a part, plus mask, pass through a ViT to get a vector. 
- take the PBR layers, pass through another ViT to get a vector
- Use contrastive loss (same as CLIP) to learn same embeddings for matching texture-patch pairs. 
[Michael - Feasibility study]
  - possibly we dont have enough input. 


--- Above is retreival from (any) set of tectures. 

Addition: 
How can there be a descriptor for a **subspace** of materials? (for a procedural material)
  - Is a particular material inthe space spanned by a procedural material
    - Sample many from procemodel
    - Thin the samples - space is all pts within DIST of nearest sample. 
    - Carve out space heirarchically (KD tree) of the descriptors. 
    
Validation: 
   - We sample MatFuse conditioned on "Wood" e.g. and use that as the subspace
   - Maybe consider using the raw matsynth textures and build e.g. a KDTree. may be dense enough for Pt+Dist. 
   - Revisit if we can sample from actual procmod
   

Step 2 [Maybe, not yet!]:   Add this vector as conditioner for MatFuse process. 




Where to submit:
  - 3DV (Aug) 
  - ICLR (Sep)


- Material Data Limitations: Address the challenge of limited material data ...
  - Can we find a better way to use the material data we have?
  - [Social Pressure Not to do this] Is a diffusion model really better than a GAN for generating PBR material? 
    - Consistancy Model ... like GAN in that you can be lucky to get tresultsin one step. hard to train. 
    - Rectified FLow ... also alt. 
  - It seems like we can tell when a (rendered) version of the material is bad. 
  - Can we find a way to use classifier based guidance? 
      - Use a differentiable render
      - Backproject the L2 error of the mean image at step T for guidance

  - Michael can add to MatSynth some procedural data (~4K) doubling about the size. 
    
- Ablation Study:
  - Show the impact of averaging CLIP vectors by comparing results with and 
    without averaging.
  - (... and other improvements discussed below)

- Automatic Cherry Picking (ACP): Implement and evaluate the effectiveness of 
  ACP by comparing results with randomly generated images versus the top-choice 
  images selected by ACP.

- More Examples: Expand the dataset of examples to demonstrate the robustness 
  and versatility of the method.

- Procedural vs Fixed Materials: Develop a method to allow the selection or 
  assignment of either procedural materials or fixed materials, aiming to 
  improve over simple CLIP vector retrieval or classifier training.

- Automatic UV Mapping: Create an automatic UV mapping solution to handle 
  rotation, scaling, and potentially translation of texture maps to ensure 
  optimal fitting.

- Clustering CLIP Vectors: Explore the possibility of clustering CLIP vectors by 
  distance threshold and specify the clustering technique. This could help in 
  grouping object parts that should share the same material.

- Multi-view Stable Diffusion: Investigate the use of multi-view Stable Diffusion 
  to generate complete and consistent textures for the entire 3D object.

- GPT for Material Descriptions: Utilize GPT models to generate detailed 
  descriptions of materials and textures to assist in the material assignment 
  process.

- Enhanced Conditioning: Include the CLIP embedding of the original prompt 
  (e.g., "a comfortable chair") along with the CLIP embeddings used to condition 
  MatFuse, potentially using a weighted combination (e.g., 0.1 * CLIP_SD + 
  CLIP_crop).

- Generate Texture Descriptors: Develop texture descriptors that are invariant 
  to 3D form and lighting and can be computed from a masked-out region. 
  (By training perhaps)

- Tileable Materials: Ensure that the generated materials are tileable to improve 
  their usability in various applications.

- Comparison with Existing Methods: Ensure that the method is compared against 
  state-of-the-art methods like MatAtlas to highlight improvements and unique 
  contributions.
    
\end{verbatim}
