# Supplementary material for: MatCLIP: Light- and Shape-Insensitive Assignment of PBR Material Models
Source: arXiv:2501.15981 source file (2025-08-09)
Supplement: Supplementary file 2 [file results_flux_bag.tex]

\newcommand{\imgwidth}{0.1325}
\newcommand{\imgskip}{0.5mm}
\newcommand{\tupleskip}{4mm}

\newcommand{\imageflux}[1]{\includegraphics[width=\imgwidth\textwidth]{#1}}
\newcommand{\imageours}[1]{\includegraphics[width=\imgwidth\textwidth]{#1}}

\begin{figure*}
	\centering
	\begin{tabular}{@{}c@{\hskip \imgskip}c@{\hspace{\tupleskip}}c@{\hskip \imgskip}c@{\hspace{\tupleskip}}c@{\hskip \imgskip}c@{}}
		Flux & MatCLIP & Flux & MatCLIP & Flux & MatCLIP \\
		\imageflux{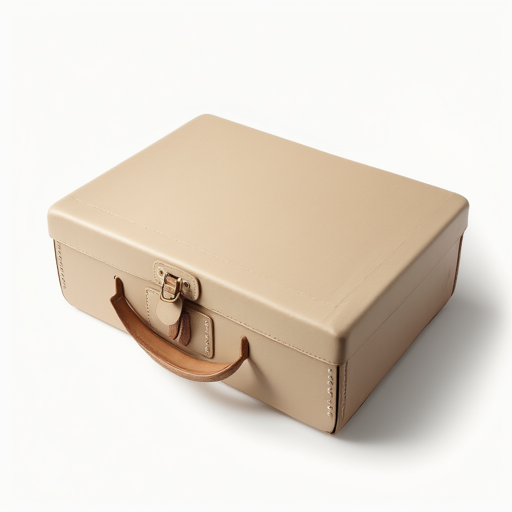} &
		\imageours{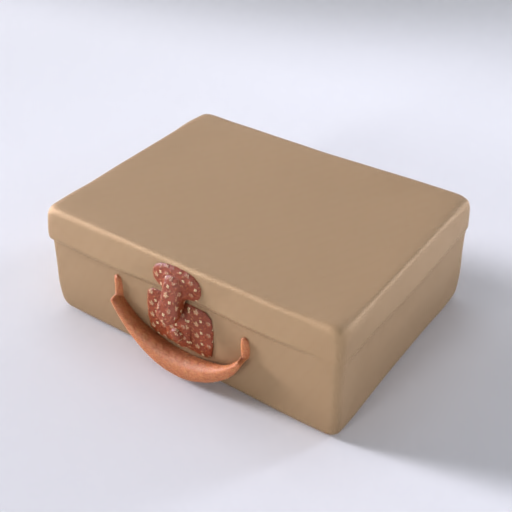} &
		\imageflux{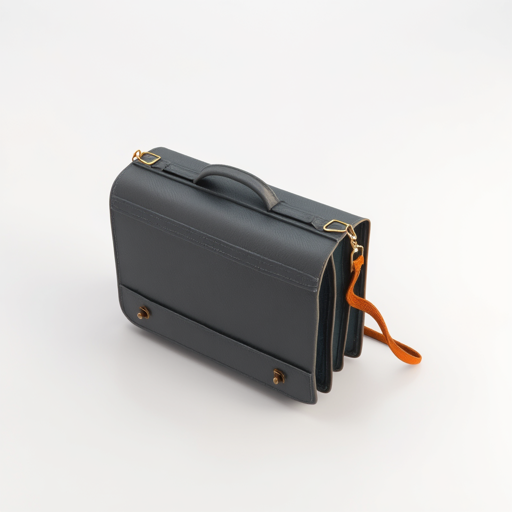} &
		\imageours{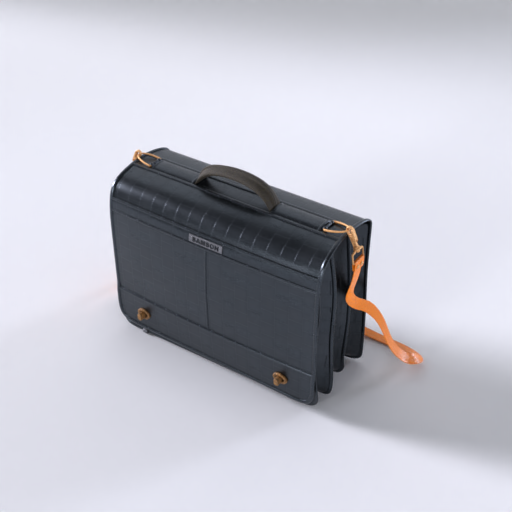} &
		\imageflux{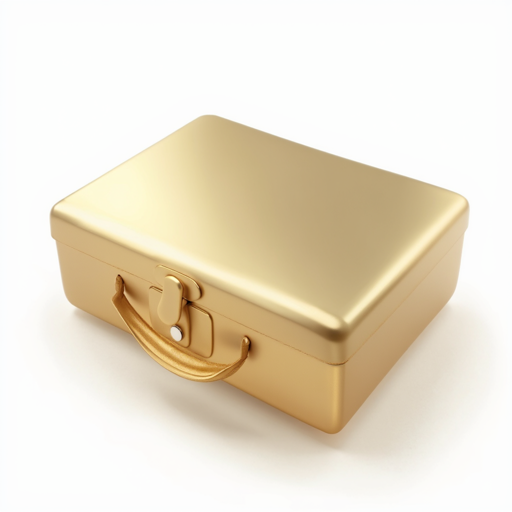} &
		\imageours{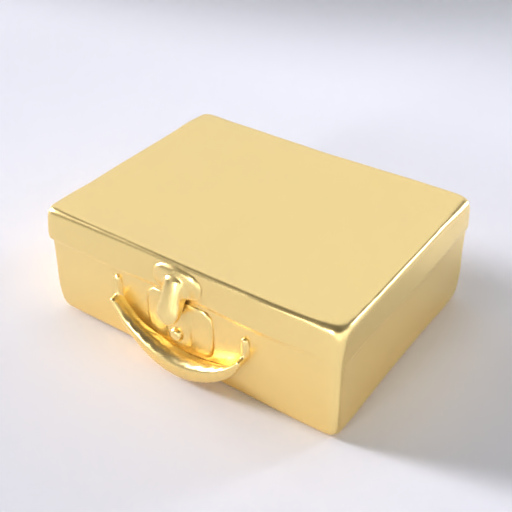} \\
		\imageflux{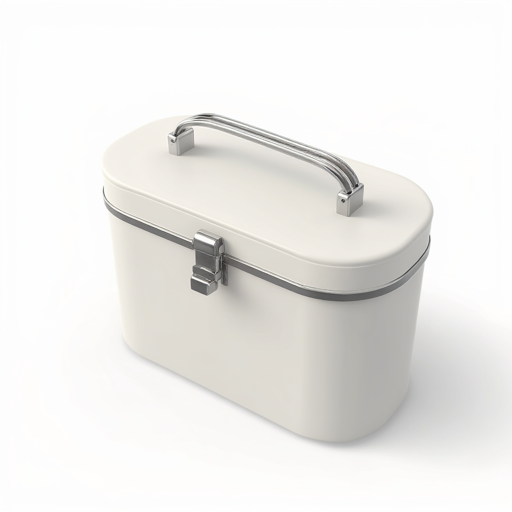} &
		\imageours{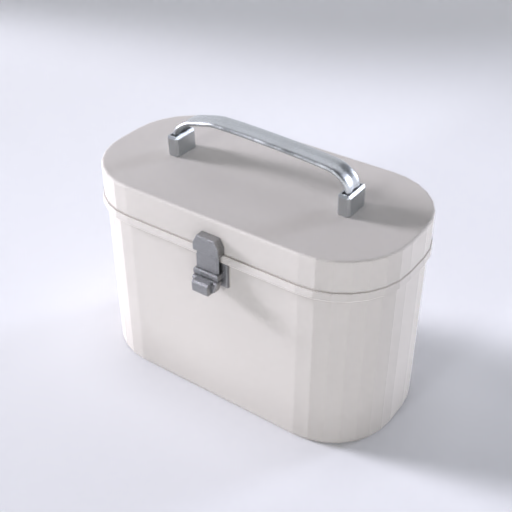} &
		\imageflux{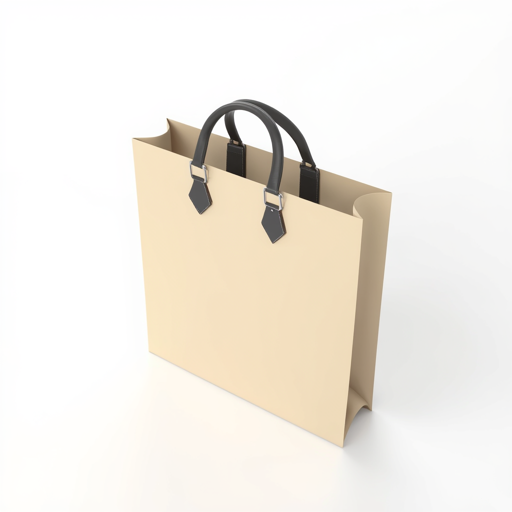} &
		\imageours{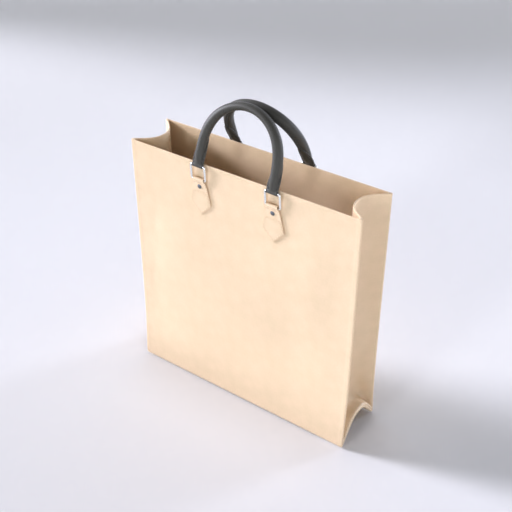} &
		\imageflux{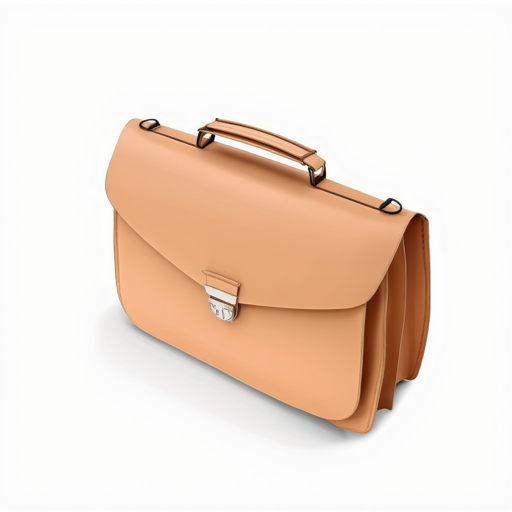} &
		\imageours{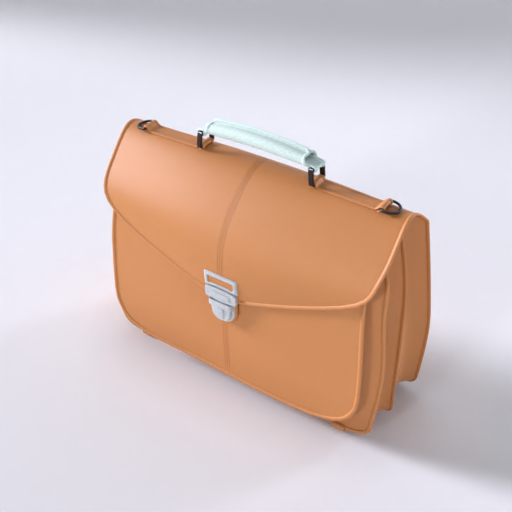} \\
		% \imageflux{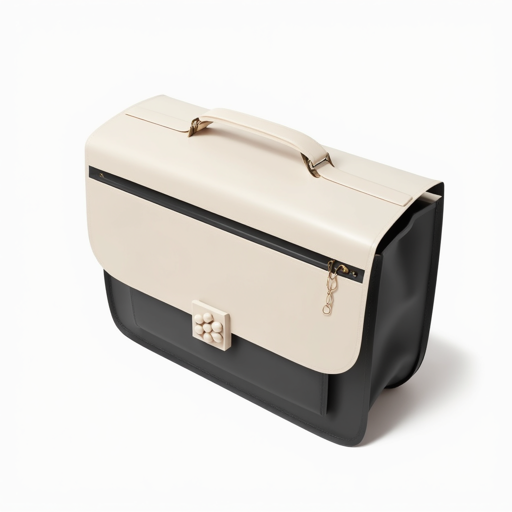} &
		% \imageours{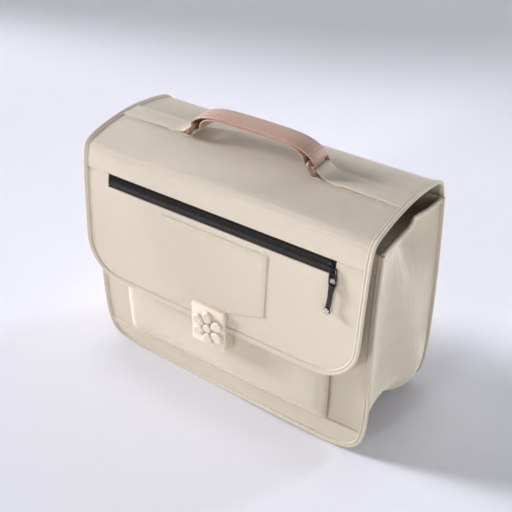} &
        \imageflux{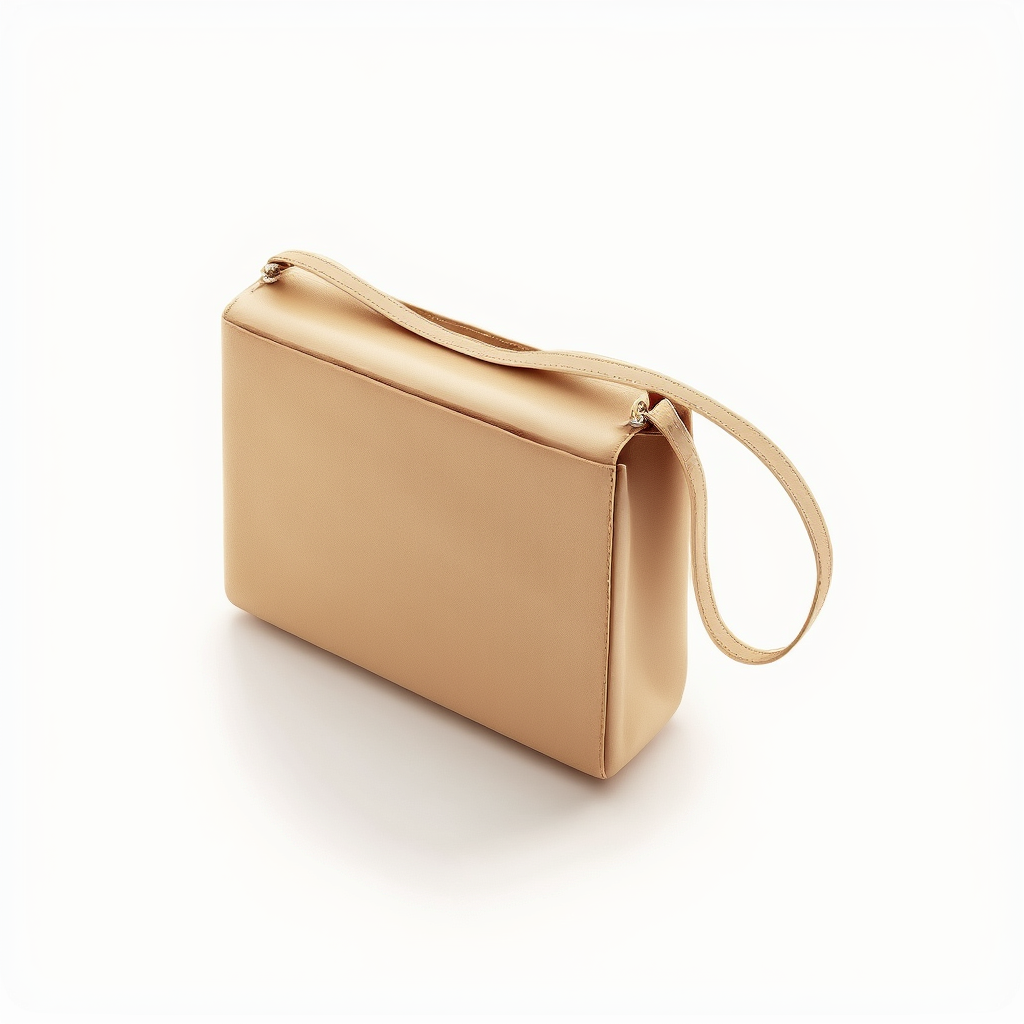} &
		\imageours{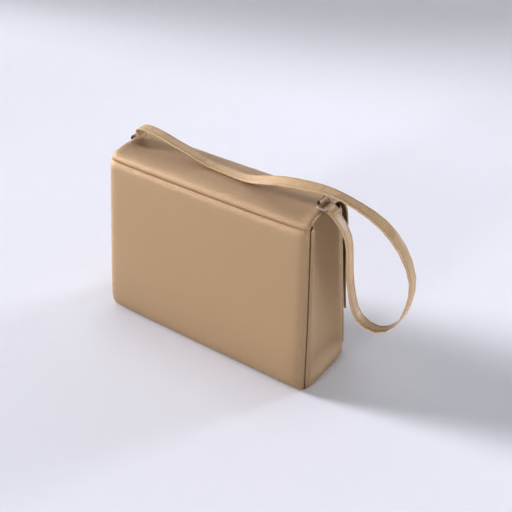} &
		% \imageflux{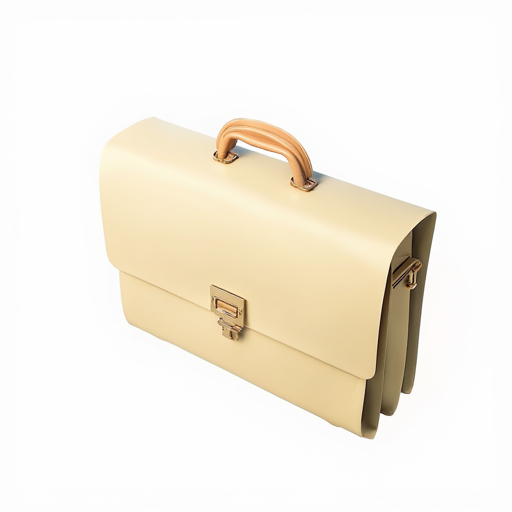} &
		% \imageours{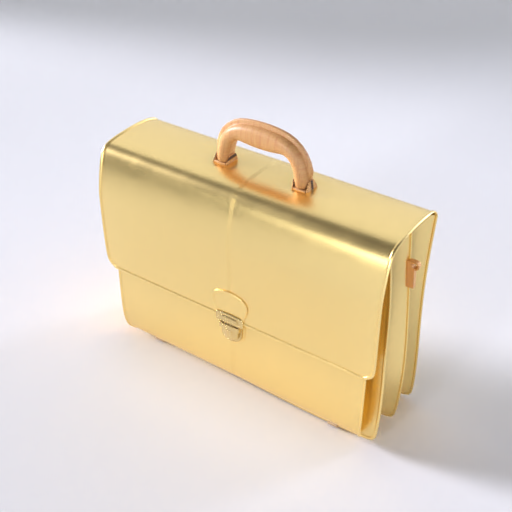} &
        \imageflux{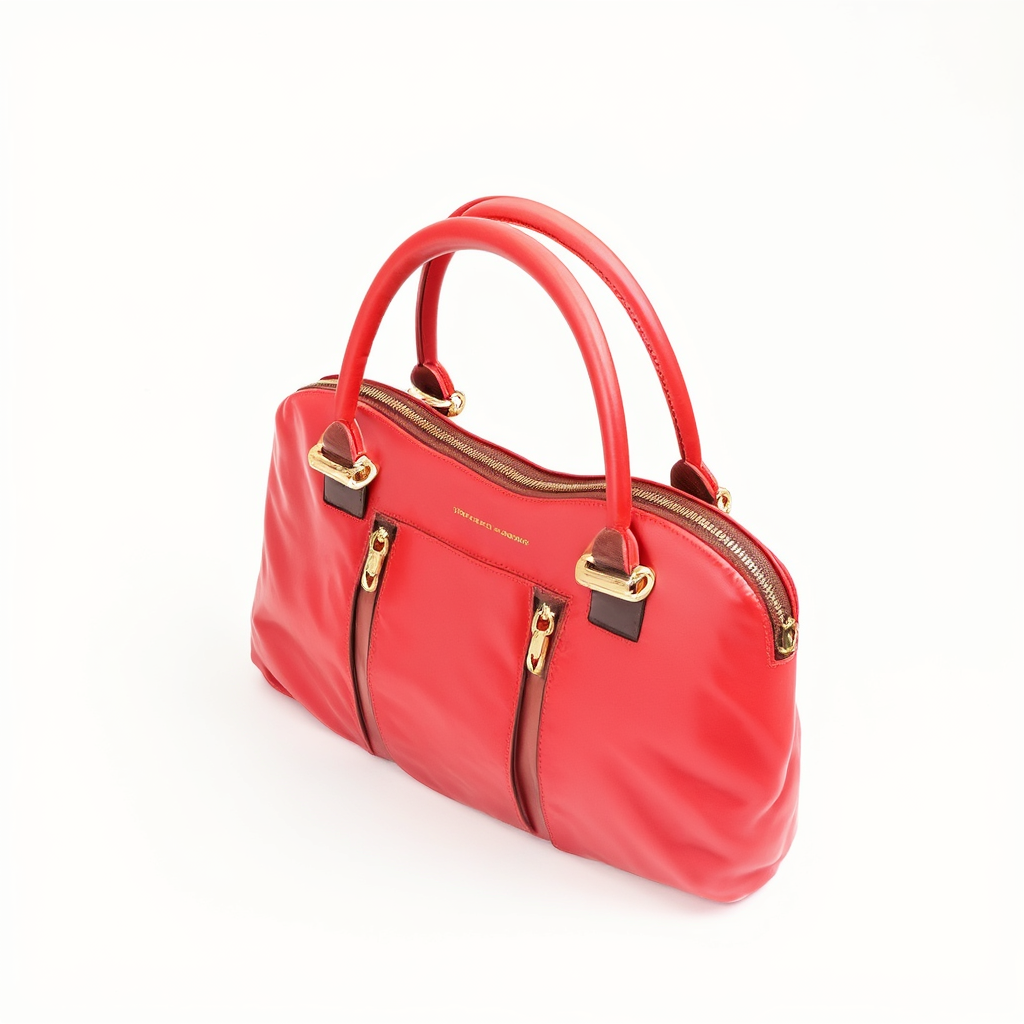} &
		\imageours{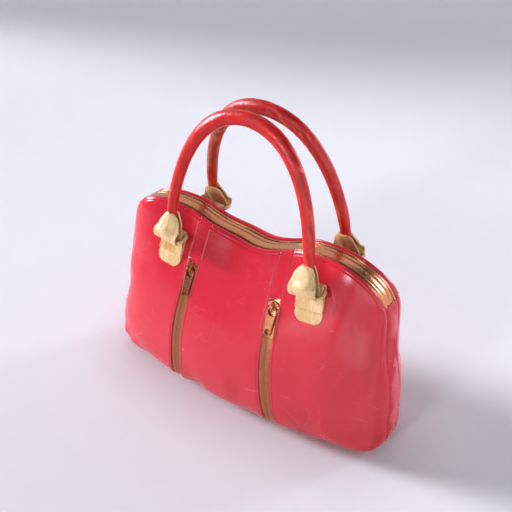} &
		\imageflux{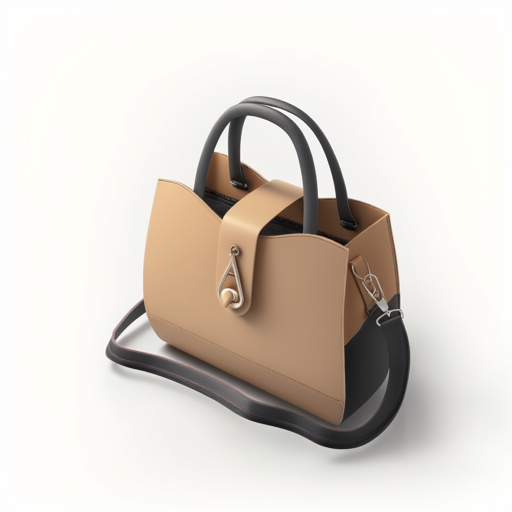} &
		\imageours{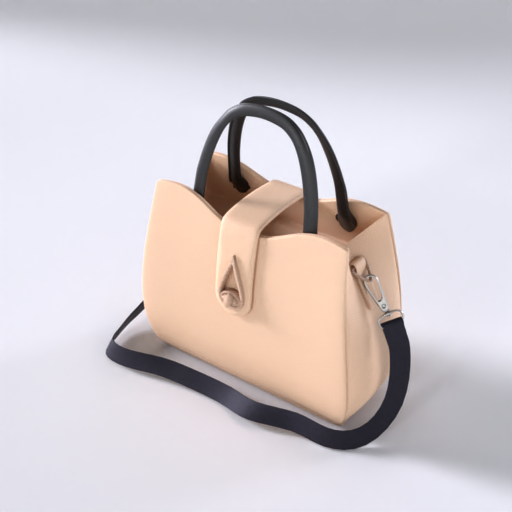} \\
		\imageflux{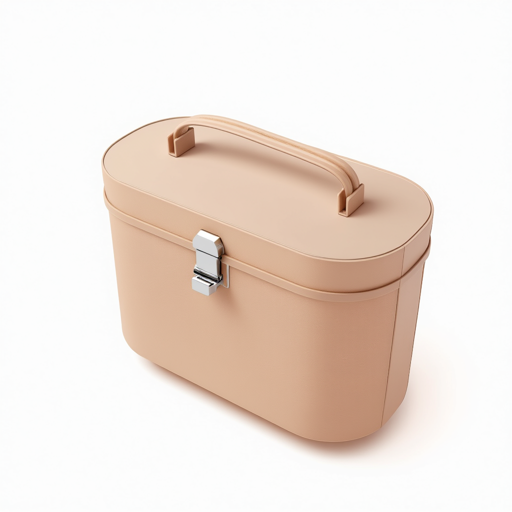} &
		\imageours{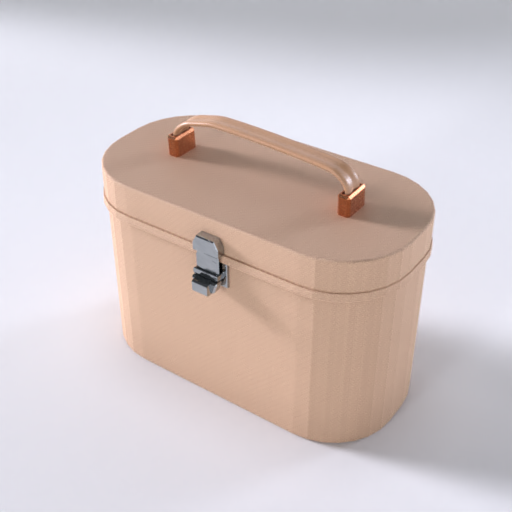} &
		\imageflux{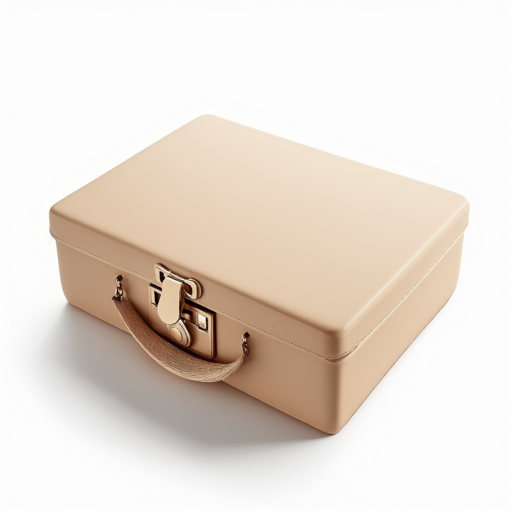} &
		\imageours{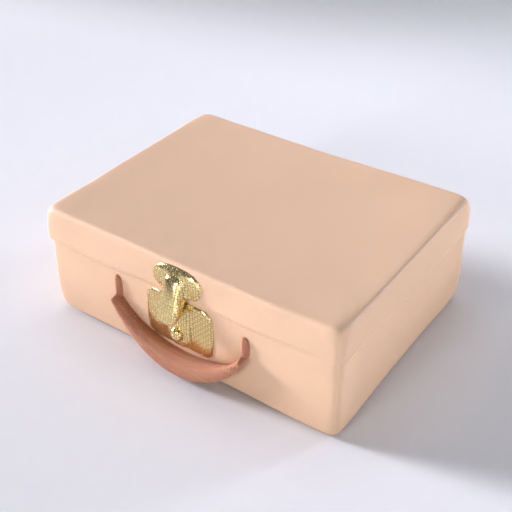} &
		\imageflux{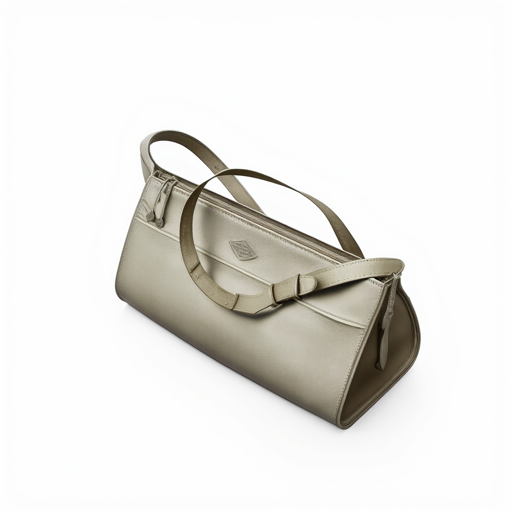} &
		\imageours{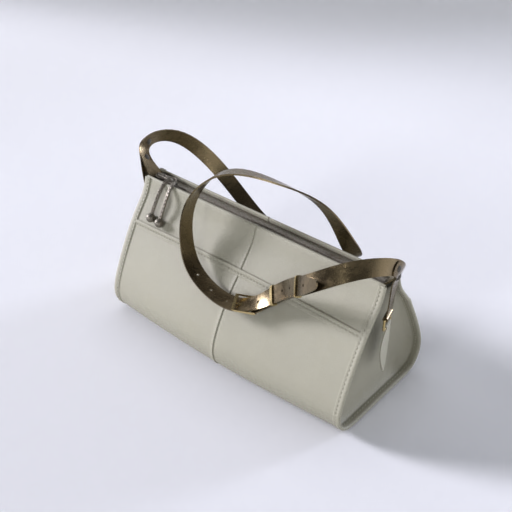} \\
		\imageflux{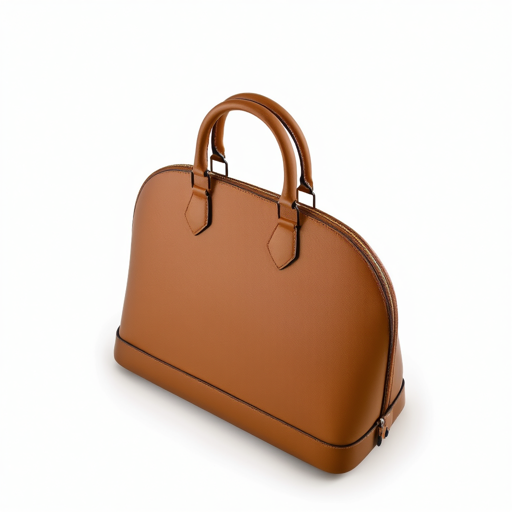} &
		\imageours{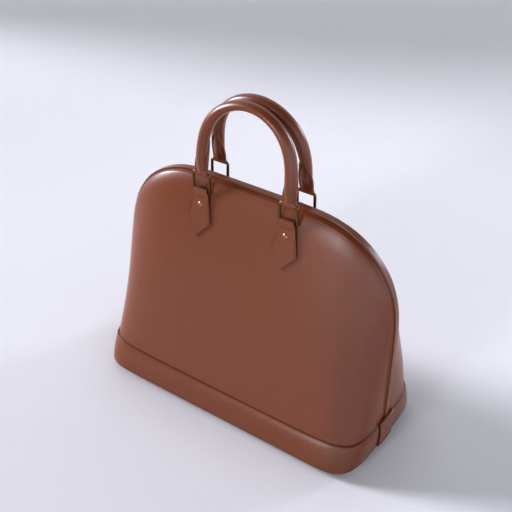} &
		\imageflux{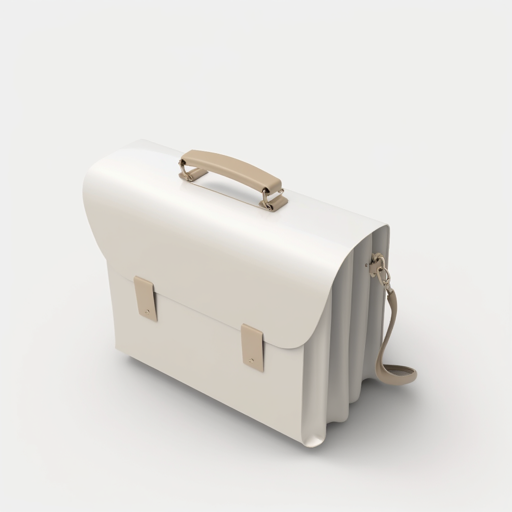} &
		\imageours{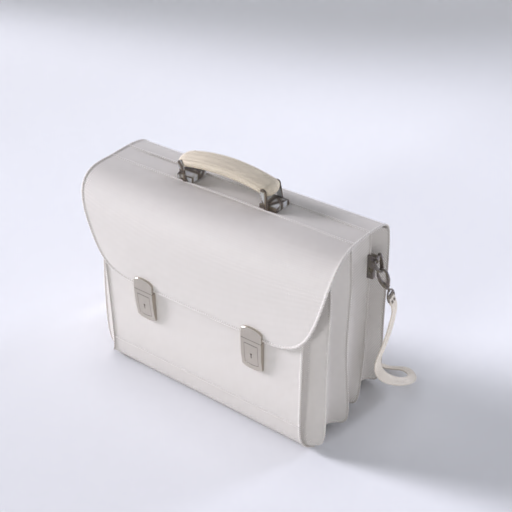} &
		\imageflux{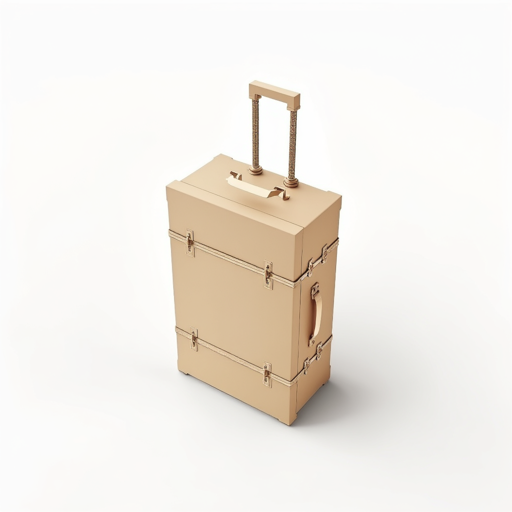} &
		\imageours{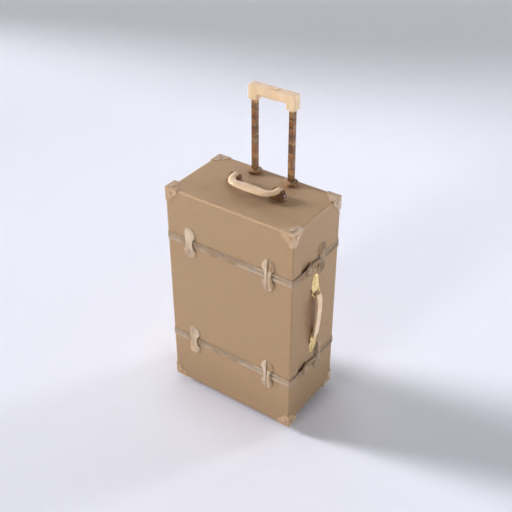} \\
		\imageflux{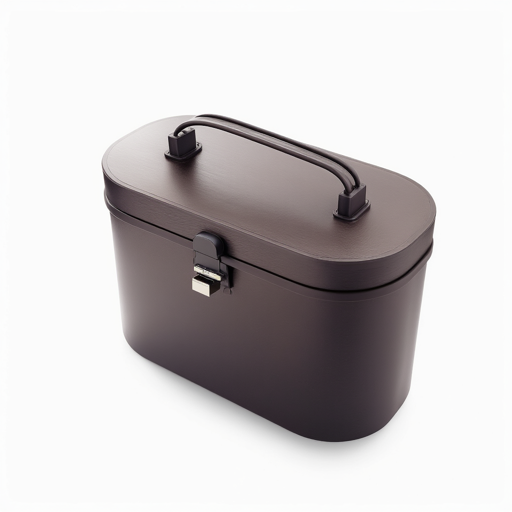} &
		\imageours{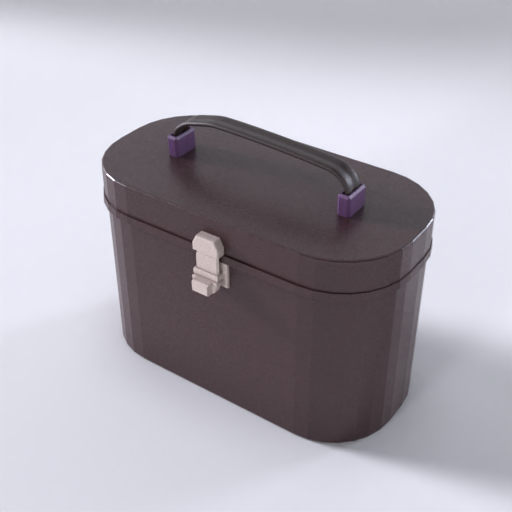} &
		\imageflux{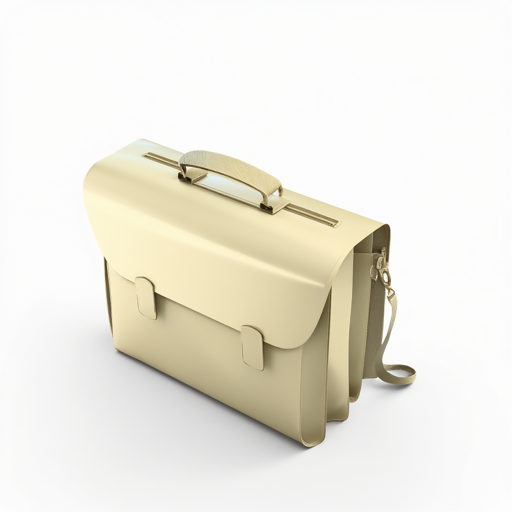} &
		\imageours{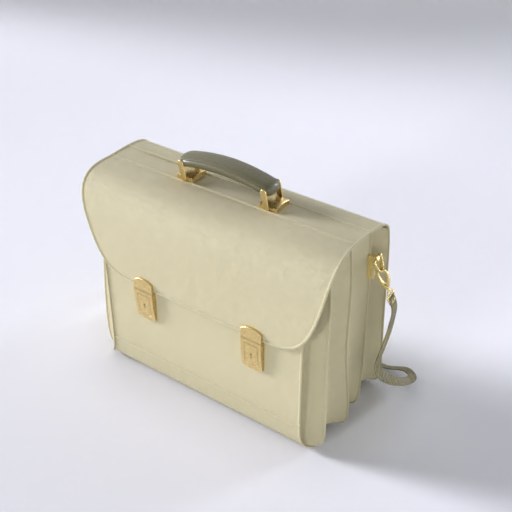} &
		\imageflux{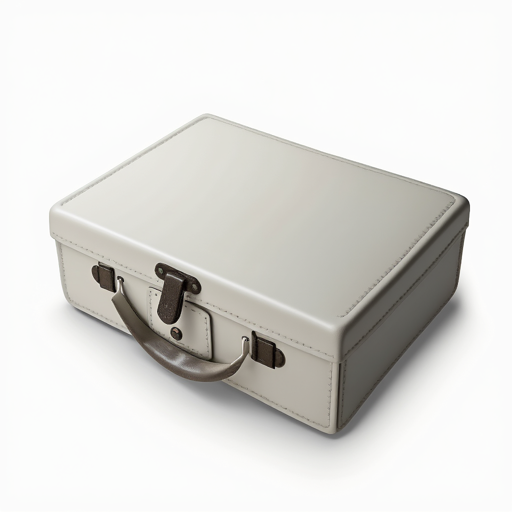} &
		\imageours{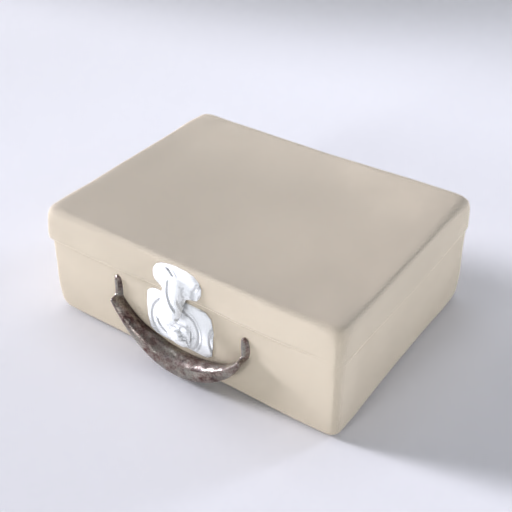} \\
		\imageflux{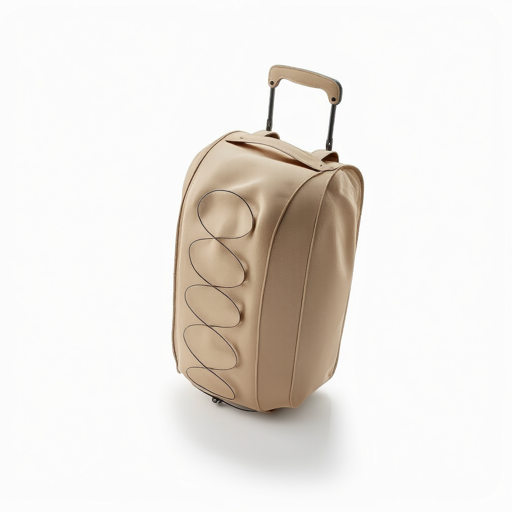} &
		\imageours{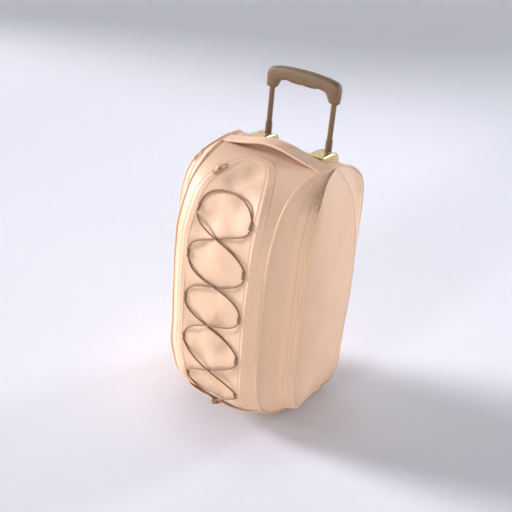} &
		\imageflux{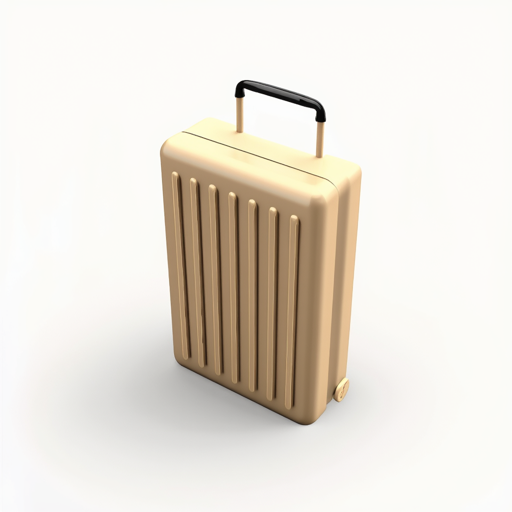} &
		\imageours{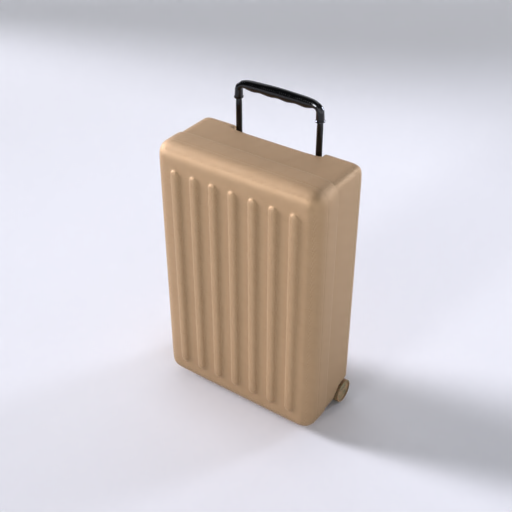} &
		\imageflux{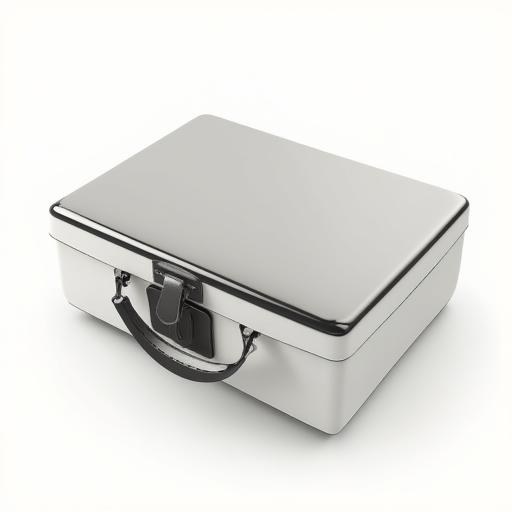} &
		\imageours{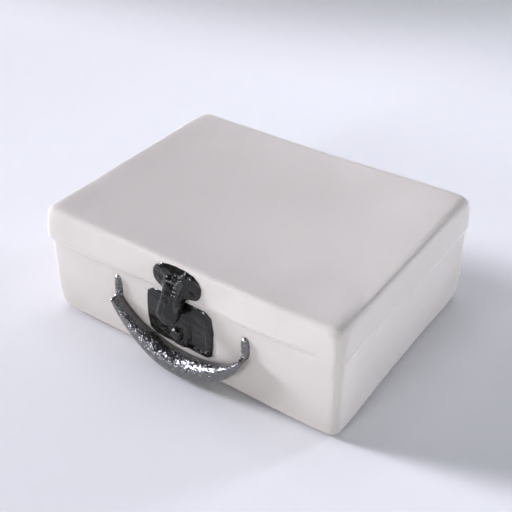} \\
		\imageflux{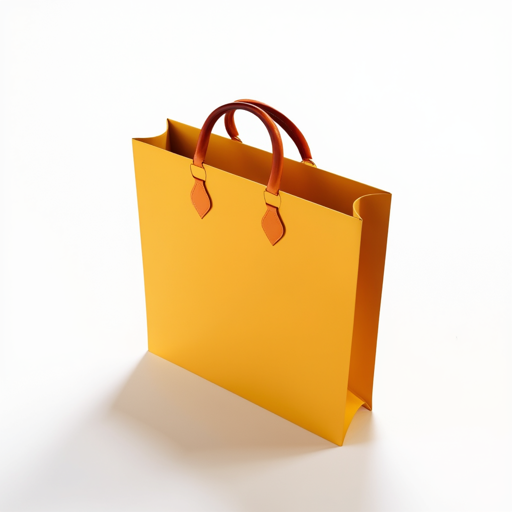} &
		\imageours{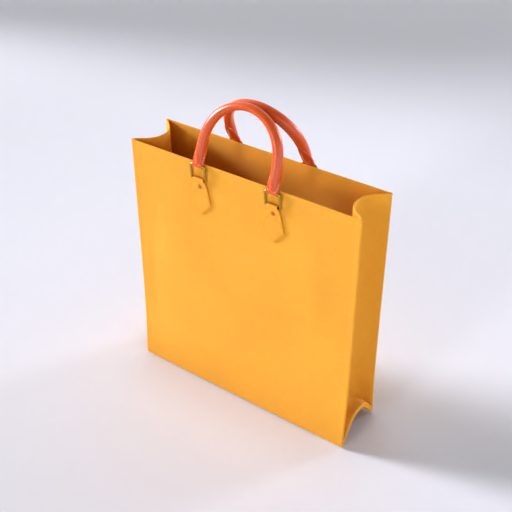} &
		\imageflux{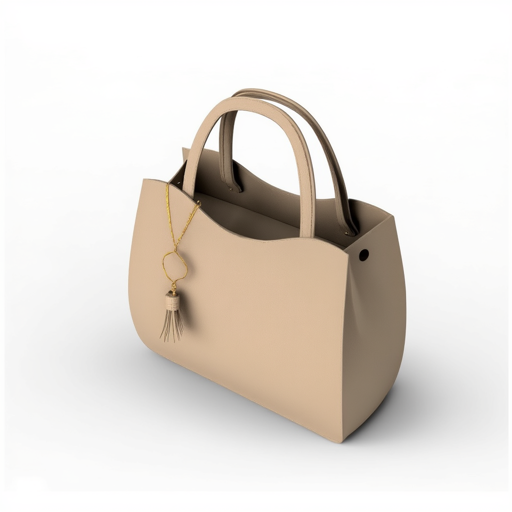} &
		\imageours{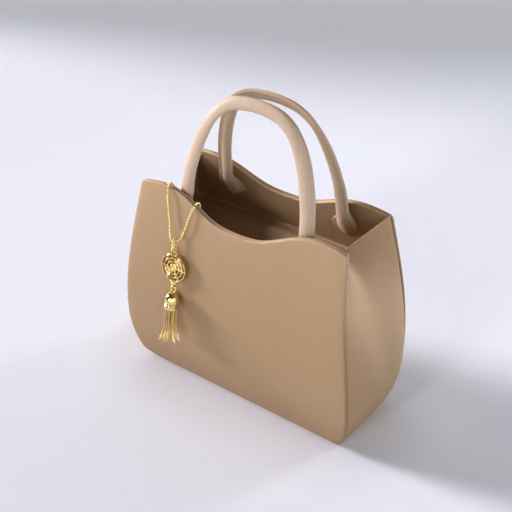} &
		\imageflux{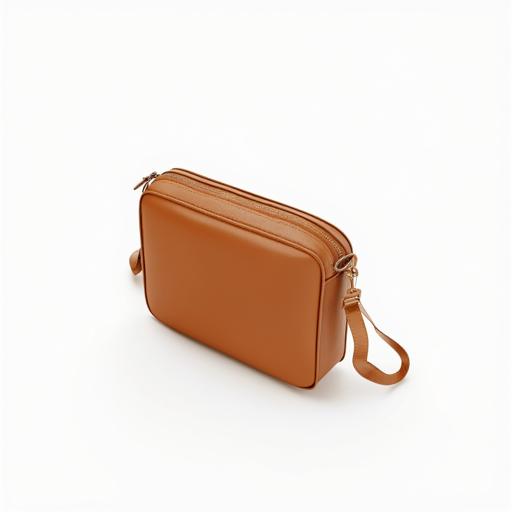} &
		\imageours{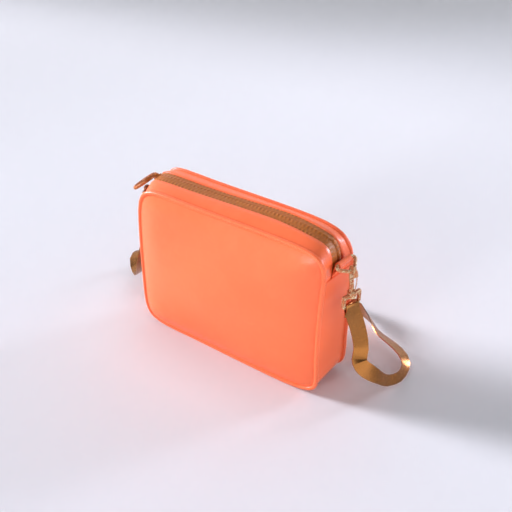} \\
	\end{tabular}
	\caption{Material matching results using MatCLIP on bag images generated by Flux \cite{flux2023}.}
	\label{fig:results_flux_bag}
\end{figure*}
