# Supplementary material for: MatCLIP: Light- and Shape-Insensitive Assignment of PBR Material Models
Source: arXiv:2501.15981 source file (2025-08-09)
Supplement: Supplementary file 5 [file generalization_lighting.tex]

\begin{table*}[t]
\centering
\begin{tabular}{lcc}
\toprule
\textbf{Method} & \textbf{Top-1 Accuracy [\%] $\uparrow$} & \textbf{Top-5 Accuracy [\%] $\uparrow$} \\
\midrule
PhotoShape (ResNet-34) & 18.83 & 35.19 \\
PhotoShape (ResNet-50) & 20.67 & 37.31 \\
PhotoShape (ViT-B/16) & 19.70 & 35.41 \\
\midrule
OpenCLIP (Max. Inscribed Square Crop, Max. Score to 42 Material Features) & 12.63 & 22.89 \\
OpenCLIP (Max. Inscribed Square Crop, Avg. Material Features) & 13.70 & 24.28 \\
\midrule
MatAtlas (0.8 × LAB + 0.2 × CLIP, Max. Score to 42 Material Features) & 11.97 & 23.43 \\
MatAtlas (0.8 × LAB + 0.2 × CLIP, Avg. Material Features) & 6.62 & 14.71 \\
\midrule
\textbf{MatCLIP (Ours)} & \textbf{35.31} & \textbf{51.90} \\
\bottomrule
\end{tabular}
\caption{
Generalization to unseen lighting conditions. We compare to variants of PhotoShape \cite{photoshape2018}, simple crop matching using CLIP \cite{radford2021_clip}, and variants of the core method of MatAtlas \cite{matatlas2024}. We either average or identify the max. score across the 42 material features of each of our materials in case of CLIP and MatAtlas. Accuracy is evaluated on Top-1 and Top-5 metrics, with higher values indicating better performance.
}
\label{tab:table_generalization_lighting}
\end{table*}
