# Supplementary material for: MatCLIP: Light- and Shape-Insensitive Assignment of PBR Material Models
Source: arXiv:2501.15981 source file (2025-08-09)
Supplement: Supplementary file 6 [file generalization_shapes.tex]

\begin{table*}[t]
\centering
\begin{tabular}{lcc}
\toprule
\textbf{Method} & \textbf{Top-1 Accuracy [\%] $\uparrow$} & \textbf{Top-5 Accuracy [\%] $\uparrow$} \\
\midrule
PhotoShape (ResNet-34) & 36.63 & 59.19 \\
PhotoShape (ResNet-50) & 38.71 & 61.42 \\
PhotoShape (ViT-B/16) & 40.42 & 62.22 \\
\midrule
OpenCLIP (Max. Inscribed Square Crop, Max. Score to 42 Material Features) & 13.56 & 26.15 \\
OpenCLIP (Max. Inscribed Square Crop, Avg. Material Features) & 16.07 & 29.28 \\
\midrule
MatAtlas (0.8 × LAB + 0.2 × CLIP, Max. Score to 42 Material Features) & 14.20 & 28.50 \\
MatAtlas (0.8 × LAB + 0.2 × CLIP, Avg. Material Features) & 9.03 & 20.93 \\
\midrule
\textbf{MatCLIP (Ours)} & \textbf{54.74} & \textbf{73.22} \\
\bottomrule
\end{tabular}
\caption{
Generalization to unseen shape categories. We compare to variants of PhotoShape \cite{photoshape2018}, simple crop matching using CLIP \cite{radford2021_clip}, and variants of the core method of MatAtlas \cite{matatlas2024}. We either average or identify the max. score across the 42 material features of each of our materials in case of CLIP and MatAtlas. Accuracy is evaluated on Top-1 and Top-5 metrics, with higher values indicating better performance.
}
\label{tab:table_generalization_shapes}
\end{table*}
